# Supplementary material for: Effect of "dipolar-biasing" on the tunability of tunneling magnetoresistance in transition metal oxide systems
Source: arXiv:1310.1466 source file (2013-10-05)

# $(LSMO)_{0.7}$ - $(CFO)_{0.3}$ EDS mapping (APL supplementary material)

The SEM-EDS mapping images, on the next page, show the distribution of elements Mn, Fe, Sr, Co and La over the area shown in the SEM-electron image (top left). The characteristic X-ray wavelength that is used for this analysis is also mentioned beside the symbol for the element. It is clearly observed from the mapping images of Fe and Co that the large slightly dark crystallites (labeled L in the electron image) are of LSMO while the CFO crystallites are smaller. The SEM image combined with the elemental mapping suggests that the LSMO and CFO grains are uniformly and randomly distributed in our composite pellets. It is to be noted that some of the LSMO crystallites could very well be small.

This EDS mapping analysis has been performed on a Zeiss microscope equipped with Oxford XMAX EDS detector and analyzer.

# $(LSMO)_{0.7}$ - $(CFO)_{0.3}$ EDS mapping (APL supplementary material)

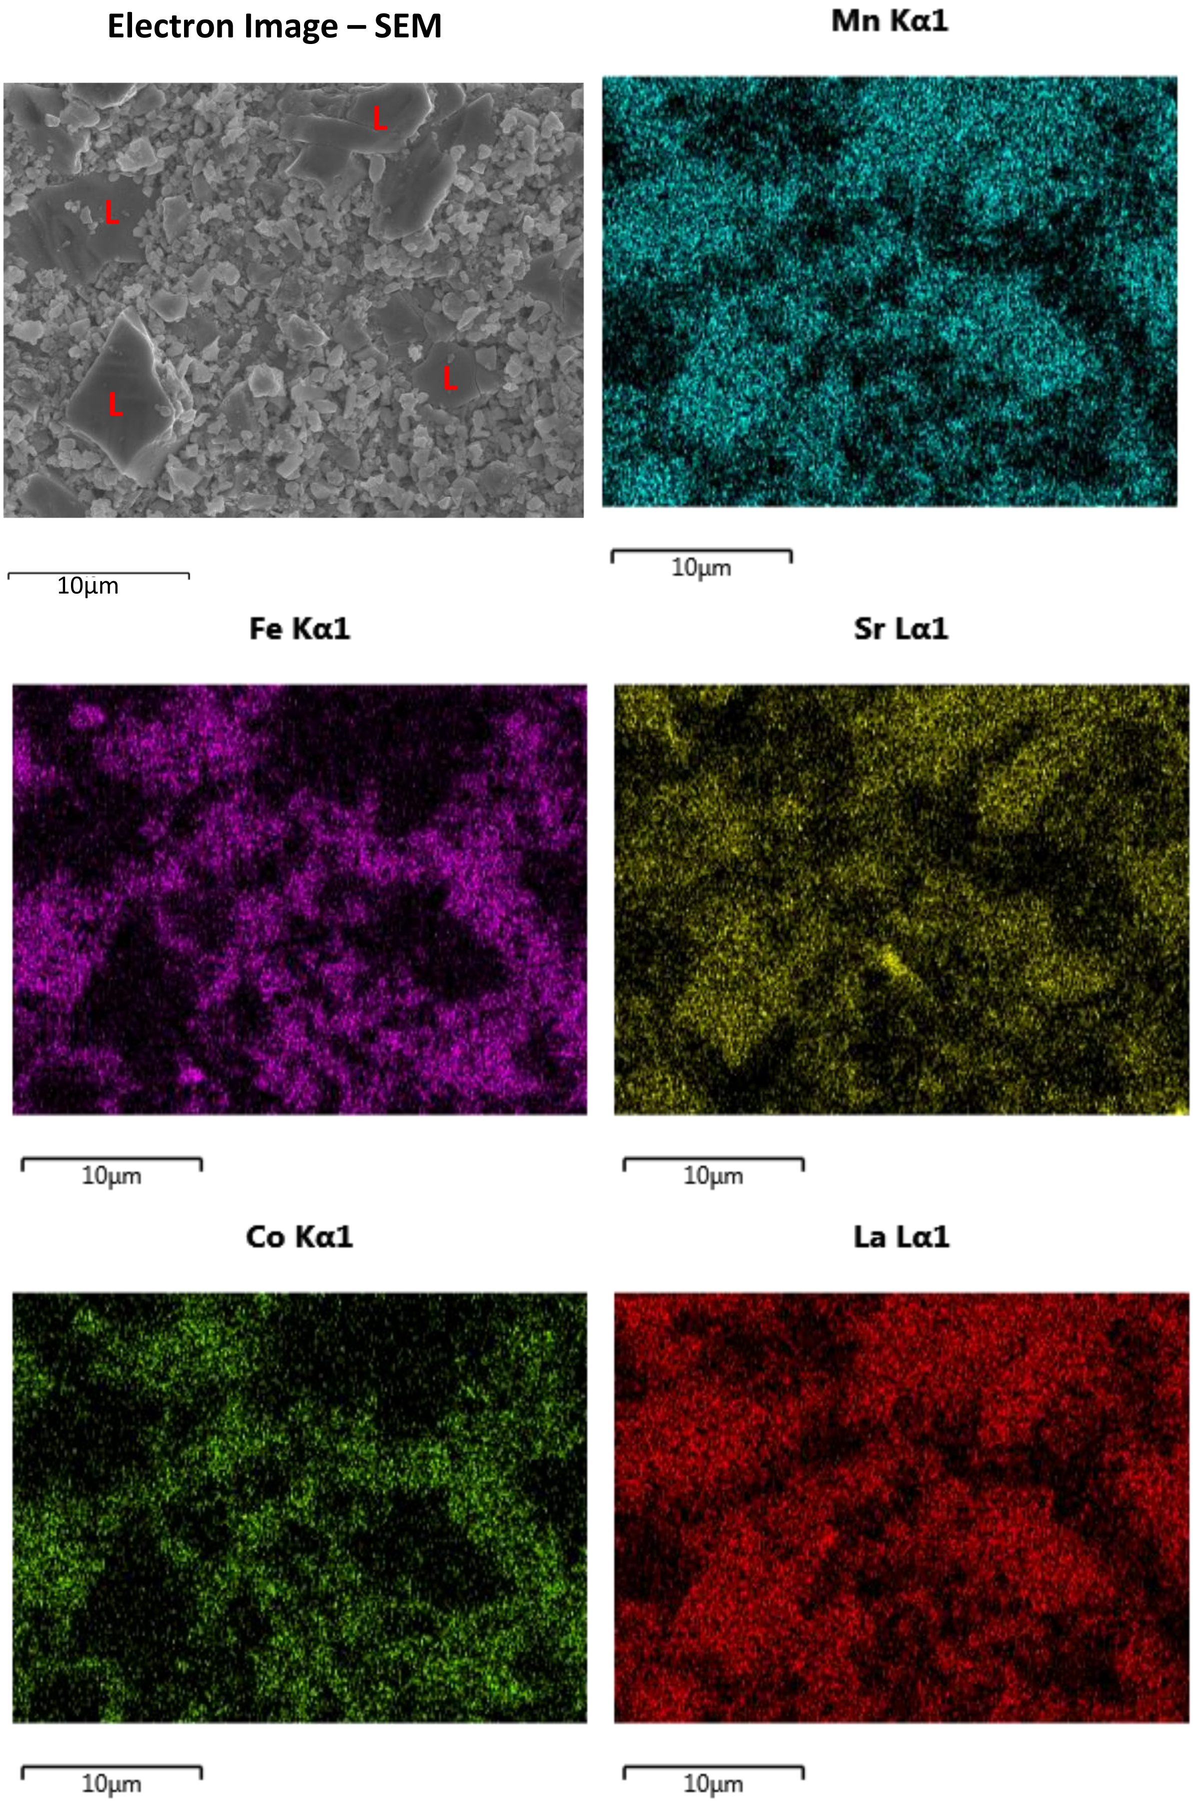

Supplement: Supplementary file 1 [file LSMO-CFO-7030_EDSmapping-SI.pdf]
